# Supplementary material for: Semantic Segmentation with Generative Models: Semi-Supervised Learning and Strong Out-of-Domain Generalization
Source: arXiv:2104.05833 source file (2021-04-12)
Supplement: Supplementary file 2 [file cxr-opt.tex]

\begin{figure*}[h!]
\begin{adjustbox}{width=0.9\linewidth, center}
\footnotesize
\addtolength{\tabcolsep}{-4pt}
\begin{tabular}{ccccccccc}
GT & Step 0 & Step 25 & Step 50 & Step 75 & Step 100 & Step 150 & Step 200 & Step 400\\

%\rotatebox{90}{\scriptsize \hspace{-1mm}In-Domain}
%&
\includegraphics[width=0.125\linewidth]{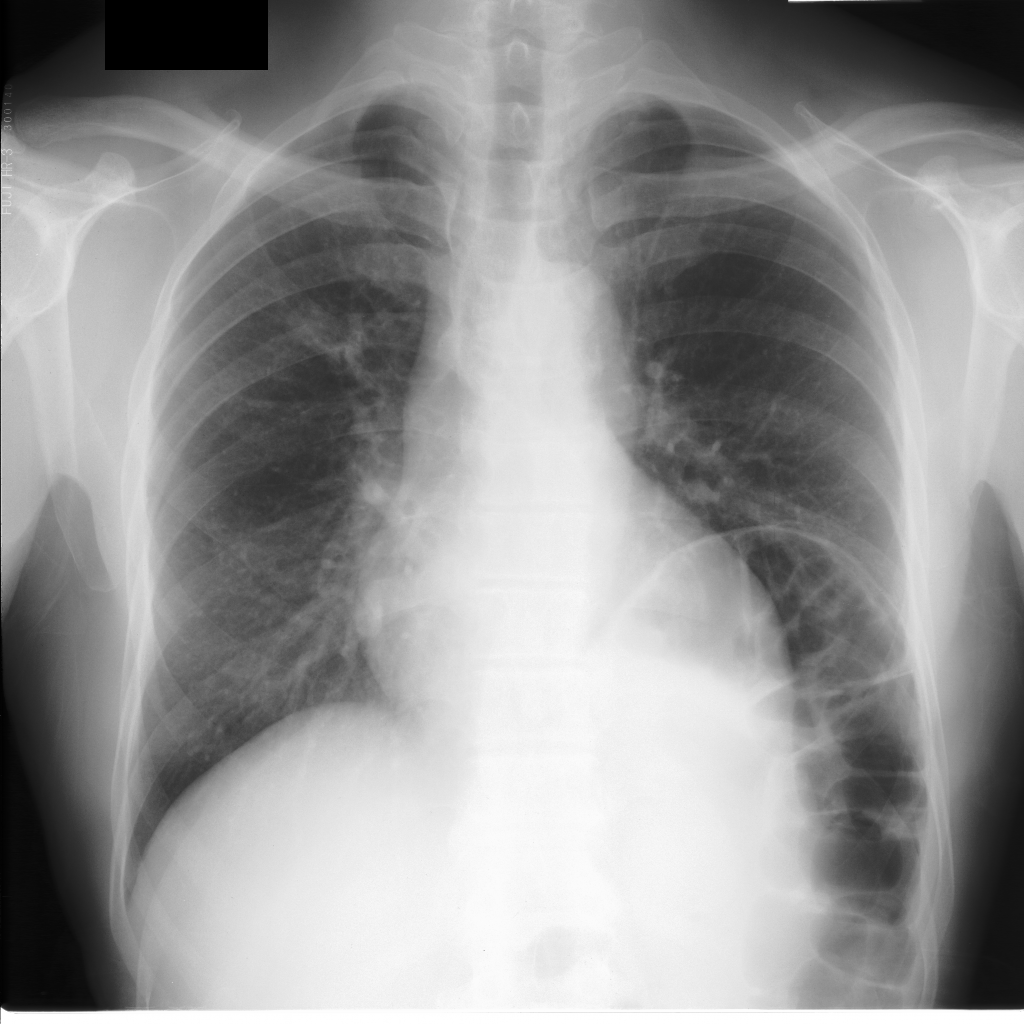}
&
\includegraphics[width=0.125\linewidth]{figures/cxr/steps/JPCLN016/img_step_00000.png}
&
\includegraphics[width=0.125\linewidth]{figures/cxr/steps/JPCLN016/img_step_00025.png}
&
\includegraphics[width=0.125\linewidth]{figures/cxr/steps/JPCLN016/img_step_00050.png}
&
\includegraphics[width=0.125\linewidth]{figures/cxr/steps/JPCLN016/img_step_00075.png}
&
\includegraphics[width=0.125\linewidth]{figures/cxr/steps/JPCLN016/img_step_00100.png}
&
\includegraphics[width=0.125\linewidth]{figures/cxr/steps/JPCLN016/img_step_00150.png}
&
\includegraphics[width=0.125\linewidth]{figures/cxr/steps/JPCLN016/img_step_00200.png}
&
\includegraphics[width=0.125\linewidth]{figures/cxr/steps/JPCLN016/img_step_00400.png}
\\

\includegraphics[width=0.125\linewidth]{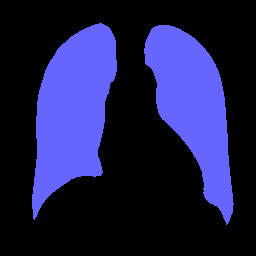}
&
\includegraphics[width=0.125\linewidth]{figures/cxr/steps/JPCLN016/label_step_00000.png}
&
\includegraphics[width=0.125\linewidth]{figures/cxr/steps/JPCLN016/label_step_00025.png}
&
\includegraphics[width=0.125\linewidth]{figures/cxr/steps/JPCLN016/label_step_00050.png}
&
\includegraphics[width=0.125\linewidth]{figures/cxr/steps/JPCLN016/label_step_00075.png}
&
\includegraphics[width=0.125\linewidth]{figures/cxr/steps/JPCLN016/label_step_00100.png}
&
\includegraphics[width=0.125\linewidth]{figures/cxr/steps/JPCLN016/label_step_00150.png}
&
\includegraphics[width=0.125\linewidth]{figures/cxr/steps/JPCLN016/label_step_00200.png}
&
\includegraphics[width=0.125\linewidth]{figures/cxr/steps/JPCLN016/label_step_00400.png}

\\
\includegraphics[width=0.125\linewidth]{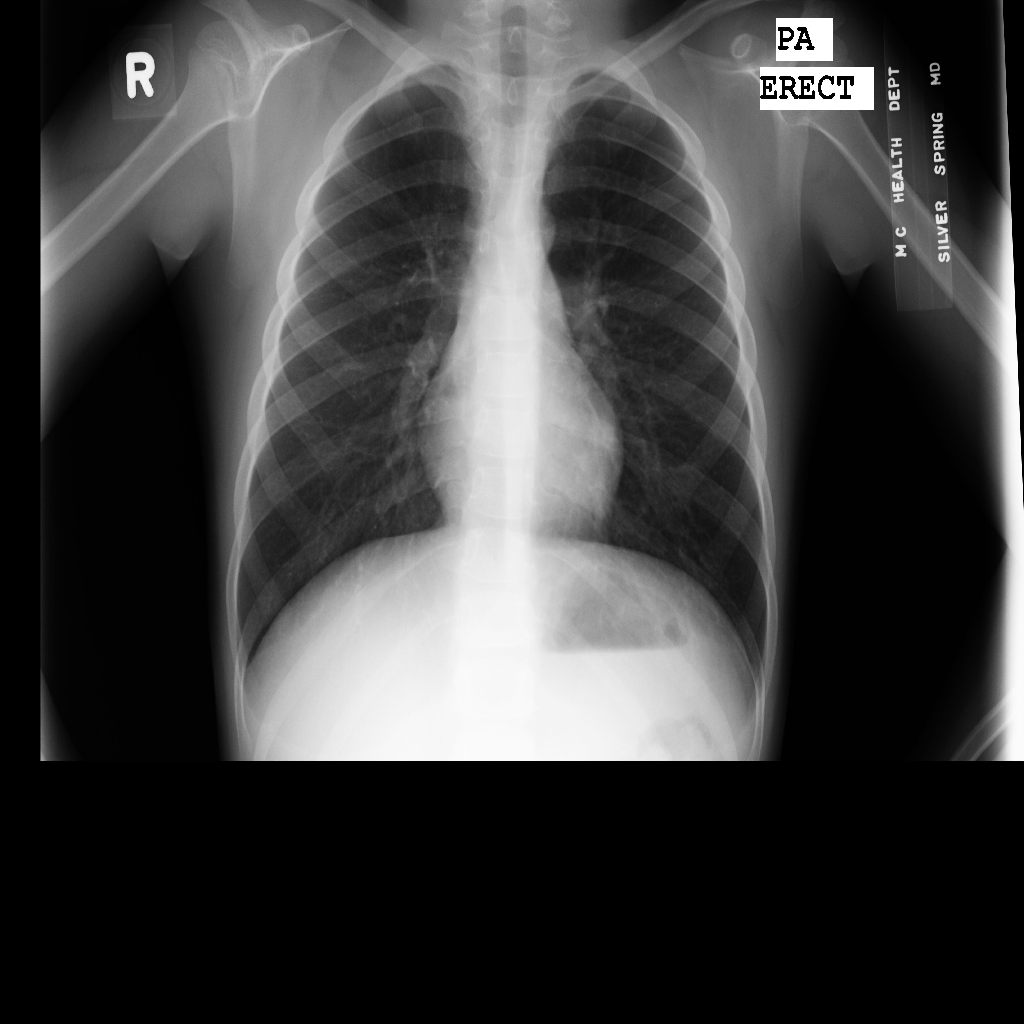}
&
\includegraphics[width=0.125\linewidth]{figures/cxr/steps/MCUCXR_0017_0/img_step_00000.png}
&
\includegraphics[width=0.125\linewidth]{figures/cxr/steps/MCUCXR_0017_0/img_step_00025.png}
&
\includegraphics[width=0.125\linewidth]{figures/cxr/steps/MCUCXR_0017_0/img_step_00050.png}
&
\includegraphics[width=0.125\linewidth]{figures/cxr/steps/MCUCXR_0017_0/img_step_00075.png}
&
\includegraphics[width=0.125\linewidth]{figures/cxr/steps/MCUCXR_0017_0/img_step_00100.png}
&
\includegraphics[width=0.125\linewidth]{figures/cxr/steps/MCUCXR_0017_0/img_step_00150.png}
&
\includegraphics[width=0.125\linewidth]{figures/cxr/steps/MCUCXR_0017_0/img_step_00200.png}
&
\includegraphics[width=0.125\linewidth]{figures/cxr/steps/MCUCXR_0017_0/img_step_00400.png}
\\

\includegraphics[width=0.125\linewidth]{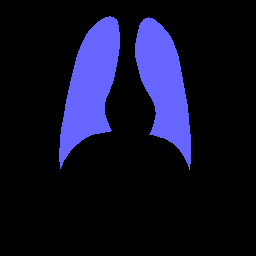}
&
\includegraphics[width=0.125\linewidth]{figures/cxr/steps/MCUCXR_0017_0/label_step_00000.png}
&
\includegraphics[width=0.125\linewidth]{figures/cxr/steps/MCUCXR_0017_0/label_step_00025.png}
&
\includegraphics[width=0.125\linewidth]{figures/cxr/steps/MCUCXR_0017_0/label_step_00050.png}
&
\includegraphics[width=0.125\linewidth]{figures/cxr/steps/MCUCXR_0017_0/label_step_00075.png}
&
\includegraphics[width=0.125\linewidth]{figures/cxr/steps/MCUCXR_0017_0/label_step_00100.png}
&
\includegraphics[width=0.125\linewidth]{figures/cxr/steps/MCUCXR_0017_0/label_step_00150.png}
&
\includegraphics[width=0.125\linewidth]{figures/cxr/steps/MCUCXR_0017_0/label_step_00200.png}
&
\includegraphics[width=0.125\linewidth]{figures/cxr/steps/MCUCXR_0017_0/label_step_00400.png}
\\

\includegraphics[width=0.125\linewidth]{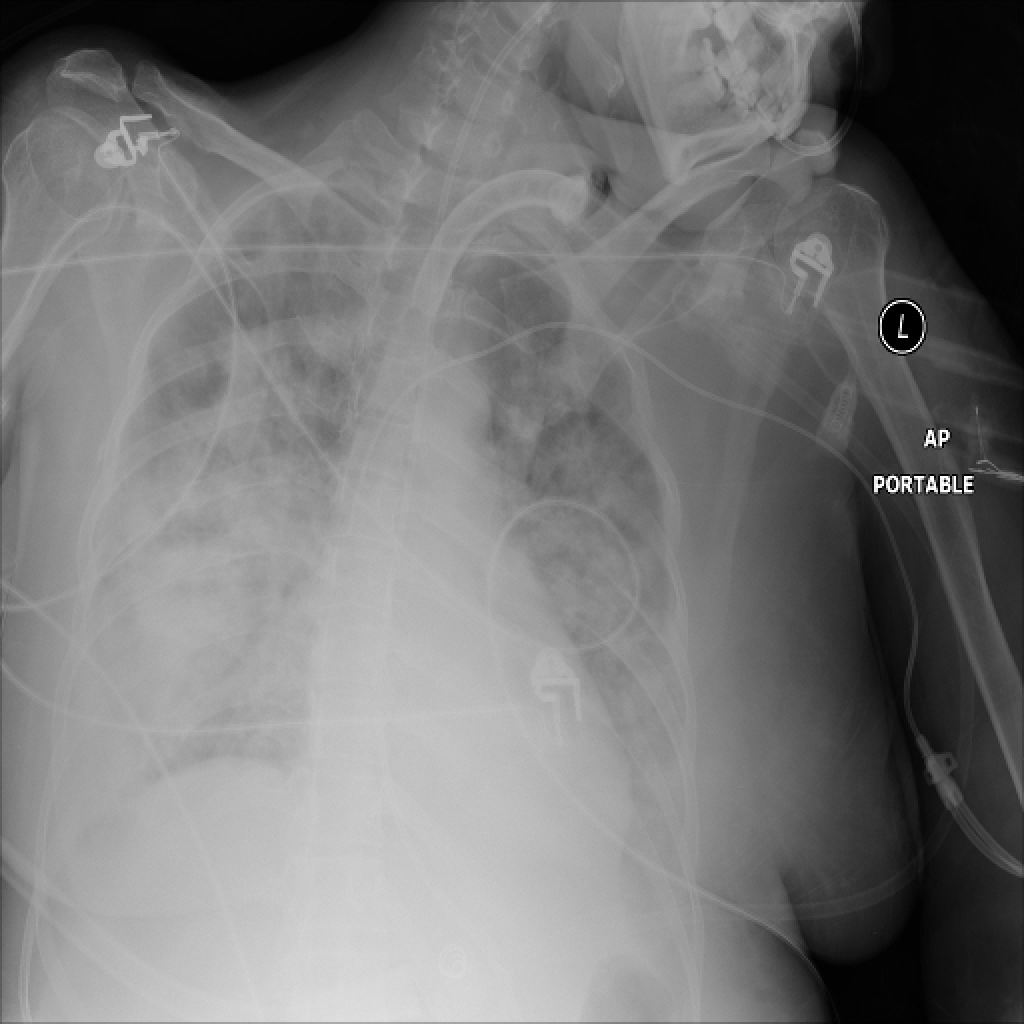}
&
\includegraphics[width=0.125\linewidth]{figures/cxr/steps/NIH_0006/img_step_00000.png}
&
\includegraphics[width=0.125\linewidth]{figures/cxr/steps/NIH_0006/img_step_00025.png}
&
\includegraphics[width=0.125\linewidth]{figures/cxr/steps/NIH_0006/img_step_00050.png}
&
\includegraphics[width=0.125\linewidth]{figures/cxr/steps/NIH_0006/img_step_00075.png}
&
\includegraphics[width=0.125\linewidth]{figures/cxr/steps/NIH_0006/img_step_00100.png}
&
\includegraphics[width=0.125\linewidth]{figures/cxr/steps/NIH_0006/img_step_00150.png}
&
\includegraphics[width=0.125\linewidth]{figures/cxr/steps/NIH_0006/img_step_00200.png}
&
\includegraphics[width=0.125\linewidth]{figures/cxr/steps/NIH_0006/img_step_00400.png}
\\

\includegraphics[width=0.125\linewidth]{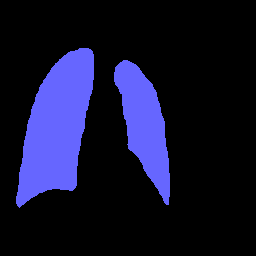}
&
\includegraphics[width=0.125\linewidth]{figures/cxr/steps/NIH_0006/label_step_00000.png}
&
\includegraphics[width=0.125\linewidth]{figures/cxr/steps/NIH_0006/label_step_00025.png}
&
\includegraphics[width=0.125\linewidth]{figures/cxr/steps/NIH_0006/label_step_00050.png}
&
\includegraphics[width=0.125\linewidth]{figures/cxr/steps/NIH_0006/label_step_00075.png}
&
\includegraphics[width=0.125\linewidth]{figures/cxr/steps/NIH_0006/label_step_00100.png}
&
\includegraphics[width=0.125\linewidth]{figures/cxr/steps/NIH_0006/label_step_00150.png}
&
\includegraphics[width=0.125\linewidth]{figures/cxr/steps/NIH_0006/label_step_00200.png}
&
\includegraphics[width=0.125\linewidth]{figures/cxr/steps/NIH_0006/label_step_00400.png}
\\

\end{tabular}
\end{adjustbox}

\caption{\footnotesize \textbf{Chest X-ray Segmentation Optimization.} Qualitative examples for reconstructions and segmentation label predictions at different optimization steps. Step 0 means using the latent code predicted by the encoder without any iterative optimization.}
\label{fig:cxr-opt}
\end{figure*}
