# Supplementary material for: Semantic Segmentation with Generative Models: Semi-Supervised Learning and Strong Out-of-Domain Generalization
Source: arXiv:2104.05833 source file (2021-04-12)
Supplement: Supplementary file 3 [file face-cariface-interp.tex]

\begin{figure*}[h!]
\begin{adjustbox}{width=0.9\linewidth, center}
\footnotesize
\addtolength{\tabcolsep}{-4pt}
\begin{tabular}{ccccccccccc}
Start & $1/10$ & $2/10$ & $3/10$ & $4/10$ & $5/10$ & $6/10$ & $7/10$ & $8/10$ & $9/10$ & End \\

%\rotatebox{90}{\scriptsize \hspace{-1mm}In-Domain}
%&
\includegraphics[width=0.125\linewidth]{figures/face/cariface-interp/sample_Bingbing Fan_C00001/img_start.png}
&
\includegraphics[width=0.125\linewidth]{figures/face/cariface-interp/sample_Bingbing Fan_C00001/img_step_0100.png}
&
\includegraphics[width=0.125\linewidth]{figures/face/cariface-interp/sample_Bingbing Fan_C00001/img_step_0200.png}
&
\includegraphics[width=0.125\linewidth]{figures/face/cariface-interp/sample_Bingbing Fan_C00001/img_step_0300.png}
&
\includegraphics[width=0.125\linewidth]{figures/face/cariface-interp/sample_Bingbing Fan_C00001/img_step_0400.png}
&
\includegraphics[width=0.125\linewidth]{figures/face/cariface-interp/sample_Bingbing Fan_C00001/img_step_0500.png}
&
\includegraphics[width=0.125\linewidth]{figures/face/cariface-interp/sample_Bingbing Fan_C00001/img_step_0600.png}
&
\includegraphics[width=0.125\linewidth]{figures/face/cariface-interp/sample_Bingbing Fan_C00001/img_step_0700.png}
&
\includegraphics[width=0.125\linewidth]{figures/face/cariface-interp/sample_Bingbing Fan_C00001/img_step_0800.png}
&
\includegraphics[width=0.125\linewidth]{figures/face/cariface-interp/sample_Bingbing Fan_C00001/img_step_0900.png}
&
\includegraphics[width=0.125\linewidth]{figures/face/cariface-interp/sample_Bingbing Fan_C00001/img_end.png}
\\

\includegraphics[width=0.125\linewidth]{figures/face/cariface-interp/sample_Bingbing Fan_C00001/seg_start.png}
&
\includegraphics[width=0.125\linewidth]{figures/face/cariface-interp/sample_Bingbing Fan_C00001/seg_step_0100.png}
&
\includegraphics[width=0.125\linewidth]{figures/face/cariface-interp/sample_Bingbing Fan_C00001/seg_step_0200.png}
&
\includegraphics[width=0.125\linewidth]{figures/face/cariface-interp/sample_Bingbing Fan_C00001/seg_step_0300.png}
&
\includegraphics[width=0.125\linewidth]{figures/face/cariface-interp/sample_Bingbing Fan_C00001/seg_step_0400.png}
&
\includegraphics[width=0.125\linewidth]{figures/face/cariface-interp/sample_Bingbing Fan_C00001/seg_step_0500.png}
&
\includegraphics[width=0.125\linewidth]{figures/face/cariface-interp/sample_Bingbing Fan_C00001/seg_step_0600.png}
&
\includegraphics[width=0.125\linewidth]{figures/face/cariface-interp/sample_Bingbing Fan_C00001/seg_step_0700.png}
&
\includegraphics[width=0.125\linewidth]{figures/face/cariface-interp/sample_Bingbing Fan_C00001/seg_step_0800.png}
&
\includegraphics[width=0.125\linewidth]{figures/face/cariface-interp/sample_Bingbing Fan_C00001/seg_step_0900.png}
&
\includegraphics[width=0.125\linewidth]{figures/face/cariface-interp/sample_Bingbing Fan_C00001/seg_end.png}

\\
\includegraphics[width=0.125\linewidth]{figures/face/cariface-interp/sample_Lucille Ball_C00001/img_start.png}
&
\includegraphics[width=0.125\linewidth]{figures/face/cariface-interp/sample_Lucille Ball_C00001/img_step_0100.png}
&
\includegraphics[width=0.125\linewidth]{figures/face/cariface-interp/sample_Lucille Ball_C00001/img_step_0200.png}
&
\includegraphics[width=0.125\linewidth]{figures/face/cariface-interp/sample_Lucille Ball_C00001/img_step_0300.png}
&
\includegraphics[width=0.125\linewidth]{figures/face/cariface-interp/sample_Lucille Ball_C00001/img_step_0400.png}
&
\includegraphics[width=0.125\linewidth]{figures/face/cariface-interp/sample_Lucille Ball_C00001/img_step_0500.png}
&
\includegraphics[width=0.125\linewidth]{figures/face/cariface-interp/sample_Lucille Ball_C00001/img_step_0600.png}
&
\includegraphics[width=0.125\linewidth]{figures/face/cariface-interp/sample_Lucille Ball_C00001/img_step_0700.png}
&
\includegraphics[width=0.125\linewidth]{figures/face/cariface-interp/sample_Lucille Ball_C00001/img_step_0800.png}
&
\includegraphics[width=0.125\linewidth]{figures/face/cariface-interp/sample_Lucille Ball_C00001/img_step_0900.png}
&
\includegraphics[width=0.125\linewidth]{figures/face/cariface-interp/sample_Lucille Ball_C00001/img_end.png}
\\

\includegraphics[width=0.125\linewidth]{figures/face/cariface-interp/sample_Lucille Ball_C00001/seg_start.png}
&
\includegraphics[width=0.125\linewidth]{figures/face/cariface-interp/sample_Lucille Ball_C00001/seg_step_0100.png}
&
\includegraphics[width=0.125\linewidth]{figures/face/cariface-interp/sample_Lucille Ball_C00001/seg_step_0200.png}
&
\includegraphics[width=0.125\linewidth]{figures/face/cariface-interp/sample_Lucille Ball_C00001/seg_step_0300.png}
&
\includegraphics[width=0.125\linewidth]{figures/face/cariface-interp/sample_Lucille Ball_C00001/seg_step_0400.png}
&
\includegraphics[width=0.125\linewidth]{figures/face/cariface-interp/sample_Lucille Ball_C00001/seg_step_0500.png}
&
\includegraphics[width=0.125\linewidth]{figures/face/cariface-interp/sample_Lucille Ball_C00001/seg_step_0600.png}
&
\includegraphics[width=0.125\linewidth]{figures/face/cariface-interp/sample_Lucille Ball_C00001/seg_step_0700.png}
&
\includegraphics[width=0.125\linewidth]{figures/face/cariface-interp/sample_Lucille Ball_C00001/seg_step_0800.png}
&
\includegraphics[width=0.125\linewidth]{figures/face/cariface-interp/sample_Lucille Ball_C00001/seg_step_0900.png}
&
\includegraphics[width=0.125\linewidth]{figures/face/cariface-interp/sample_Lucille Ball_C00001/seg_end.png}

\\

\includegraphics[width=0.125\linewidth]{figures/face/cariface-interp/sample_Harry Potter_C00001/img_start.png}
&
\includegraphics[width=0.125\linewidth]{figures/face/cariface-interp/sample_Harry Potter_C00001/img_step_0100.png}
&
\includegraphics[width=0.125\linewidth]{figures/face/cariface-interp/sample_Harry Potter_C00001/img_step_0200.png}
&
\includegraphics[width=0.125\linewidth]{figures/face/cariface-interp/sample_Harry Potter_C00001/img_step_0300.png}
&
\includegraphics[width=0.125\linewidth]{figures/face/cariface-interp/sample_Harry Potter_C00001/img_step_0400.png}
&
\includegraphics[width=0.125\linewidth]{figures/face/cariface-interp/sample_Harry Potter_C00001/img_step_0500.png}
&
\includegraphics[width=0.125\linewidth]{figures/face/cariface-interp/sample_Harry Potter_C00001/img_step_0600.png}
&
\includegraphics[width=0.125\linewidth]{figures/face/cariface-interp/sample_Harry Potter_C00001/img_step_0700.png}
&
\includegraphics[width=0.125\linewidth]{figures/face/cariface-interp/sample_Harry Potter_C00001/img_step_0800.png}
&
\includegraphics[width=0.125\linewidth]{figures/face/cariface-interp/sample_Harry Potter_C00001/img_step_0900.png}
&
\includegraphics[width=0.125\linewidth]{figures/face/cariface-interp/sample_Harry Potter_C00001/img_end.png}
\\

\includegraphics[width=0.125\linewidth]{figures/face/cariface-interp/sample_Harry Potter_C00001/seg_start.png}
&
\includegraphics[width=0.125\linewidth]{figures/face/cariface-interp/sample_Harry Potter_C00001/seg_step_0100.png}
&
\includegraphics[width=0.125\linewidth]{figures/face/cariface-interp/sample_Harry Potter_C00001/seg_step_0200.png}
&
\includegraphics[width=0.125\linewidth]{figures/face/cariface-interp/sample_Harry Potter_C00001/seg_step_0300.png}
&
\includegraphics[width=0.125\linewidth]{figures/face/cariface-interp/sample_Harry Potter_C00001/seg_step_0400.png}
&
\includegraphics[width=0.125\linewidth]{figures/face/cariface-interp/sample_Harry Potter_C00001/seg_step_0500.png}
&
\includegraphics[width=0.125\linewidth]{figures/face/cariface-interp/sample_Harry Potter_C00001/seg_step_0600.png}
&
\includegraphics[width=0.125\linewidth]{figures/face/cariface-interp/sample_Harry Potter_C00001/seg_step_0700.png}
&
\includegraphics[width=0.125\linewidth]{figures/face/cariface-interp/sample_Harry Potter_C00001/seg_step_0800.png}
&
\includegraphics[width=0.125\linewidth]{figures/face/cariface-interp/sample_Harry Potter_C00001/seg_step_0900.png}
&
\includegraphics[width=0.125\linewidth]{figures/face/cariface-interp/sample_Harry Potter_C00001/seg_end.png}

\\

\includegraphics[width=0.125\linewidth]{figures/face/cariface-interp/sample_Vladimir Putin_C00001/img_start.png}
&
\includegraphics[width=0.125\linewidth]{figures/face/cariface-interp/sample_Vladimir Putin_C00001/img_step_0100.png}
&
\includegraphics[width=0.125\linewidth]{figures/face/cariface-interp/sample_Vladimir Putin_C00001/img_step_0200.png}
&
\includegraphics[width=0.125\linewidth]{figures/face/cariface-interp/sample_Vladimir Putin_C00001/img_step_0300.png}
&
\includegraphics[width=0.125\linewidth]{figures/face/cariface-interp/sample_Vladimir Putin_C00001/img_step_0400.png}
&
\includegraphics[width=0.125\linewidth]{figures/face/cariface-interp/sample_Vladimir Putin_C00001/img_step_0500.png}
&
\includegraphics[width=0.125\linewidth]{figures/face/cariface-interp/sample_Vladimir Putin_C00001/img_step_0600.png}
&
\includegraphics[width=0.125\linewidth]{figures/face/cariface-interp/sample_Vladimir Putin_C00001/img_step_0700.png}
&
\includegraphics[width=0.125\linewidth]{figures/face/cariface-interp/sample_Vladimir Putin_C00001/img_step_0800.png}
&
\includegraphics[width=0.125\linewidth]{figures/face/cariface-interp/sample_Vladimir Putin_C00001/img_step_0900.png}
&
\includegraphics[width=0.125\linewidth]{figures/face/cariface-interp/sample_Vladimir Putin_C00001/img_end.png}
\\

\includegraphics[width=0.125\linewidth]{figures/face/cariface-interp/sample_Vladimir Putin_C00001/seg_start.png}
&
\includegraphics[width=0.125\linewidth]{figures/face/cariface-interp/sample_Vladimir Putin_C00001/seg_step_0100.png}
&
\includegraphics[width=0.125\linewidth]{figures/face/cariface-interp/sample_Vladimir Putin_C00001/seg_step_0200.png}
&
\includegraphics[width=0.125\linewidth]{figures/face/cariface-interp/sample_Vladimir Putin_C00001/seg_step_0300.png}
&
\includegraphics[width=0.125\linewidth]{figures/face/cariface-interp/sample_Vladimir Putin_C00001/seg_step_0400.png}
&
\includegraphics[width=0.125\linewidth]{figures/face/cariface-interp/sample_Vladimir Putin_C00001/seg_step_0500.png}
&
\includegraphics[width=0.125\linewidth]{figures/face/cariface-interp/sample_Vladimir Putin_C00001/seg_step_0600.png}
&
\includegraphics[width=0.125\linewidth]{figures/face/cariface-interp/sample_Vladimir Putin_C00001/seg_step_0700.png}
&
\includegraphics[width=0.125\linewidth]{figures/face/cariface-interp/sample_Vladimir Putin_C00001/seg_step_0800.png}
&
\includegraphics[width=0.125\linewidth]{figures/face/cariface-interp/sample_Vladimir Putin_C00001/seg_step_0900.png}
&
\includegraphics[width=0.125\linewidth]{figures/face/cariface-interp/sample_Vladimir Putin_C00001/seg_end.png}

\\

\end{tabular}
\end{adjustbox}
%\vspace{-4mm}
\caption{\footnotesize \textbf{Interpolations between Random Latent Codes and Cartoon Faces.} Linear interpolations between random latent codes and latent codes of selected Cartoons. We obtain the Cartoon latent codes by performing inverse optimization. The interpolation is done in $\mathcal{W}^+$-space. We show both the interpolated images and their semantic segmentation labels. The results show that the generative model learnt a smooth latent space with meaningful images along the interpolation path. Furthermore, we observe consistency between images and predicted labels along the interpolation path. This is noteworthy, since we are interpolating beyond the training domain.}
\label{fig:face-cari-interp}
\end{figure*}
