# Supplementary material for: Semantic Segmentation with Generative Models: Semi-Supervised Learning and Strong Out-of-Domain Generalization
Source: arXiv:2104.05833 source file (2021-04-12)
Supplement: Supplementary file 5 [file face-metface-interp.tex]

\begin{figure*}[h!]
\begin{adjustbox}{width=0.9\linewidth, center}
\footnotesize
\addtolength{\tabcolsep}{-4pt}
\begin{tabular}{ccccccccccc}
Start & $1/10$ & $2/10$ & $3/10$ & $4/10$ & $5/10$ & $6/10$ & $7/10$ & $8/10$ & $9/10$ & End \\

%\rotatebox{90}{\scriptsize \hspace{-1mm}In-Domain}
%&
\includegraphics[width=0.125\linewidth]{figures/face/metface-interp/sample_10242-00/img_start.png}
&
\includegraphics[width=0.125\linewidth]{figures/face/metface-interp/sample_10242-00/img_step_0100.png}
&
\includegraphics[width=0.125\linewidth]{figures/face/metface-interp/sample_10242-00/img_step_0200.png}
&
\includegraphics[width=0.125\linewidth]{figures/face/metface-interp/sample_10242-00/img_step_0300.png}
&
\includegraphics[width=0.125\linewidth]{figures/face/metface-interp/sample_10242-00/img_step_0400.png}
&
\includegraphics[width=0.125\linewidth]{figures/face/metface-interp/sample_10242-00/img_step_0500.png}
&
\includegraphics[width=0.125\linewidth]{figures/face/metface-interp/sample_10242-00/img_step_0600.png}
&
\includegraphics[width=0.125\linewidth]{figures/face/metface-interp/sample_10242-00/img_step_0700.png}
&
\includegraphics[width=0.125\linewidth]{figures/face/metface-interp/sample_10242-00/img_step_0800.png}
&
\includegraphics[width=0.125\linewidth]{figures/face/metface-interp/sample_10242-00/img_step_0900.png}
&
\includegraphics[width=0.125\linewidth]{figures/face/metface-interp/sample_10242-00/img_end.png}
\\

\includegraphics[width=0.125\linewidth]{figures/face/metface-interp/sample_10242-00/seg_start.png}
&
\includegraphics[width=0.125\linewidth]{figures/face/metface-interp/sample_10242-00/seg_step_0100.png}
&
\includegraphics[width=0.125\linewidth]{figures/face/metface-interp/sample_10242-00/seg_step_0200.png}
&
\includegraphics[width=0.125\linewidth]{figures/face/metface-interp/sample_10242-00/seg_step_0300.png}
&
\includegraphics[width=0.125\linewidth]{figures/face/metface-interp/sample_10242-00/seg_step_0400.png}
&
\includegraphics[width=0.125\linewidth]{figures/face/metface-interp/sample_10242-00/seg_step_0500.png}
&
\includegraphics[width=0.125\linewidth]{figures/face/metface-interp/sample_10242-00/seg_step_0600.png}
&
\includegraphics[width=0.125\linewidth]{figures/face/metface-interp/sample_10242-00/seg_step_0700.png}
&
\includegraphics[width=0.125\linewidth]{figures/face/metface-interp/sample_10242-00/seg_step_0800.png}
&
\includegraphics[width=0.125\linewidth]{figures/face/metface-interp/sample_10242-00/seg_step_0900.png}
&
\includegraphics[width=0.125\linewidth]{figures/face/metface-interp/sample_10242-00/seg_end.png}

\\
\includegraphics[width=0.125\linewidth]{figures/face/metface-interp/sample_10466-00/img_start.png}
&
\includegraphics[width=0.125\linewidth]{figures/face/metface-interp/sample_10466-00/img_step_0100.png}
&
\includegraphics[width=0.125\linewidth]{figures/face/metface-interp/sample_10466-00/img_step_0200.png}
&
\includegraphics[width=0.125\linewidth]{figures/face/metface-interp/sample_10466-00/img_step_0300.png}
&
\includegraphics[width=0.125\linewidth]{figures/face/metface-interp/sample_10466-00/img_step_0400.png}
&
\includegraphics[width=0.125\linewidth]{figures/face/metface-interp/sample_10466-00/img_step_0500.png}
&
\includegraphics[width=0.125\linewidth]{figures/face/metface-interp/sample_10466-00/img_step_0600.png}
&
\includegraphics[width=0.125\linewidth]{figures/face/metface-interp/sample_10466-00/img_step_0700.png}
&
\includegraphics[width=0.125\linewidth]{figures/face/metface-interp/sample_10466-00/img_step_0800.png}
&
\includegraphics[width=0.125\linewidth]{figures/face/metface-interp/sample_10466-00/img_step_0900.png}
&
\includegraphics[width=0.125\linewidth]{figures/face/metface-interp/sample_10466-00/img_end.png}
\\

\includegraphics[width=0.125\linewidth]{figures/face/metface-interp/sample_10466-00/seg_start.png}
&
\includegraphics[width=0.125\linewidth]{figures/face/metface-interp/sample_10466-00/seg_step_0100.png}
&
\includegraphics[width=0.125\linewidth]{figures/face/metface-interp/sample_10466-00/seg_step_0200.png}
&
\includegraphics[width=0.125\linewidth]{figures/face/metface-interp/sample_10466-00/seg_step_0300.png}
&
\includegraphics[width=0.125\linewidth]{figures/face/metface-interp/sample_10466-00/seg_step_0400.png}
&
\includegraphics[width=0.125\linewidth]{figures/face/metface-interp/sample_10466-00/seg_step_0500.png}
&
\includegraphics[width=0.125\linewidth]{figures/face/metface-interp/sample_10466-00/seg_step_0600.png}
&
\includegraphics[width=0.125\linewidth]{figures/face/metface-interp/sample_10466-00/seg_step_0700.png}
&
\includegraphics[width=0.125\linewidth]{figures/face/metface-interp/sample_10466-00/seg_step_0800.png}
&
\includegraphics[width=0.125\linewidth]{figures/face/metface-interp/sample_10466-00/seg_step_0900.png}
&
\includegraphics[width=0.125\linewidth]{figures/face/metface-interp/sample_10466-00/seg_end.png}

\\

\includegraphics[width=0.125\linewidth]{figures/face/metface-interp/sample_544709-00/img_start.png}
&
\includegraphics[width=0.125\linewidth]{figures/face/metface-interp/sample_544709-00/img_step_0100.png}
&
\includegraphics[width=0.125\linewidth]{figures/face/metface-interp/sample_544709-00/img_step_0200.png}
&
\includegraphics[width=0.125\linewidth]{figures/face/metface-interp/sample_544709-00/img_step_0300.png}
&
\includegraphics[width=0.125\linewidth]{figures/face/metface-interp/sample_544709-00/img_step_0400.png}
&
\includegraphics[width=0.125\linewidth]{figures/face/metface-interp/sample_544709-00/img_step_0500.png}
&
\includegraphics[width=0.125\linewidth]{figures/face/metface-interp/sample_544709-00/img_step_0600.png}
&
\includegraphics[width=0.125\linewidth]{figures/face/metface-interp/sample_544709-00/img_step_0700.png}
&
\includegraphics[width=0.125\linewidth]{figures/face/metface-interp/sample_544709-00/img_step_0800.png}
&
\includegraphics[width=0.125\linewidth]{figures/face/metface-interp/sample_544709-00/img_step_0900.png}
&
\includegraphics[width=0.125\linewidth]{figures/face/metface-interp/sample_544709-00/img_end.png}
\\

\includegraphics[width=0.125\linewidth]{figures/face/metface-interp/sample_544709-00/seg_start.png}
&
\includegraphics[width=0.125\linewidth]{figures/face/metface-interp/sample_544709-00/seg_step_0100.png}
&
\includegraphics[width=0.125\linewidth]{figures/face/metface-interp/sample_544709-00/seg_step_0200.png}
&
\includegraphics[width=0.125\linewidth]{figures/face/metface-interp/sample_544709-00/seg_step_0300.png}
&
\includegraphics[width=0.125\linewidth]{figures/face/metface-interp/sample_544709-00/seg_step_0400.png}
&
\includegraphics[width=0.125\linewidth]{figures/face/metface-interp/sample_544709-00/seg_step_0500.png}
&
\includegraphics[width=0.125\linewidth]{figures/face/metface-interp/sample_544709-00/seg_step_0600.png}
&
\includegraphics[width=0.125\linewidth]{figures/face/metface-interp/sample_544709-00/seg_step_0700.png}
&
\includegraphics[width=0.125\linewidth]{figures/face/metface-interp/sample_544709-00/seg_step_0800.png}
&
\includegraphics[width=0.125\linewidth]{figures/face/metface-interp/sample_544709-00/seg_step_0900.png}
&
\includegraphics[width=0.125\linewidth]{figures/face/metface-interp/sample_544709-00/seg_end.png}

\\

\includegraphics[width=0.125\linewidth]{figures/face/metface-interp/sample_471036-00/img_start.png}
&
\includegraphics[width=0.125\linewidth]{figures/face/metface-interp/sample_471036-00/img_step_0100.png}
&
\includegraphics[width=0.125\linewidth]{figures/face/metface-interp/sample_471036-00/img_step_0200.png}
&
\includegraphics[width=0.125\linewidth]{figures/face/metface-interp/sample_471036-00/img_step_0300.png}
&
\includegraphics[width=0.125\linewidth]{figures/face/metface-interp/sample_471036-00/img_step_0400.png}
&
\includegraphics[width=0.125\linewidth]{figures/face/metface-interp/sample_471036-00/img_step_0500.png}
&
\includegraphics[width=0.125\linewidth]{figures/face/metface-interp/sample_471036-00/img_step_0600.png}
&
\includegraphics[width=0.125\linewidth]{figures/face/metface-interp/sample_471036-00/img_step_0700.png}
&
\includegraphics[width=0.125\linewidth]{figures/face/metface-interp/sample_471036-00/img_step_0800.png}
&
\includegraphics[width=0.125\linewidth]{figures/face/metface-interp/sample_471036-00/img_step_0900.png}
&
\includegraphics[width=0.125\linewidth]{figures/face/metface-interp/sample_471036-00/img_end.png}
\\

\includegraphics[width=0.125\linewidth]{figures/face/metface-interp/sample_471036-00/seg_start.png}
&
\includegraphics[width=0.125\linewidth]{figures/face/metface-interp/sample_471036-00/seg_step_0100.png}
&
\includegraphics[width=0.125\linewidth]{figures/face/metface-interp/sample_471036-00/seg_step_0200.png}
&
\includegraphics[width=0.125\linewidth]{figures/face/metface-interp/sample_471036-00/seg_step_0300.png}
&
\includegraphics[width=0.125\linewidth]{figures/face/metface-interp/sample_471036-00/seg_step_0400.png}
&
\includegraphics[width=0.125\linewidth]{figures/face/metface-interp/sample_471036-00/seg_step_0500.png}
&
\includegraphics[width=0.125\linewidth]{figures/face/metface-interp/sample_471036-00/seg_step_0600.png}
&
\includegraphics[width=0.125\linewidth]{figures/face/metface-interp/sample_471036-00/seg_step_0700.png}
&
\includegraphics[width=0.125\linewidth]{figures/face/metface-interp/sample_471036-00/seg_step_0800.png}
&
\includegraphics[width=0.125\linewidth]{figures/face/metface-interp/sample_471036-00/seg_step_0900.png}
&
\includegraphics[width=0.125\linewidth]{figures/face/metface-interp/sample_471036-00/seg_end.png}

\\

\end{tabular}
\end{adjustbox}
%\vspace{-4mm}
\caption{\footnotesize \textbf{Interpolations between Random Latent Codes and MetFaces.} Linear interpolations between random latent codes and latent codes of MetFace images. We obtain the MetFace latent codes by performing inverse optimization. The interpolation is done in $\mathcal{W}^+$-space. We show both the interpolated images and their semantic segmentation labels. The results show that the generative model learnt a smooth latent space with meaningful images along the interpolation path. Furthermore, we observe consistency between images and predicted labels along the interpolation path. This is noteworthy, since we are interpolating beyond the training domain.}
\label{fig:face-met-interp}
\end{figure*}
