# Supplementary material for: Semantic Segmentation with Generative Models: Semi-Supervised Learning and Strong Out-of-Domain Generalization
Source: arXiv:2104.05833 source file (2021-04-12)
Supplement: Supplementary file 6 [file face-opt.tex]

\begin{figure*}[t!]
\begin{adjustbox}{width=0.9\linewidth, center}
\footnotesize
\addtolength{\tabcolsep}{-4pt}
\begin{tabular}{ccccccccc}
GT & Step 0 & Step 25 & Step 50 & Step 75 & Step 100 & Step 150 & Step 200 & Step 400\\

%\rotatebox{90}{\scriptsize \hspace{-1mm}In-Domain}
%&
\includegraphics[width=0.125\linewidth]{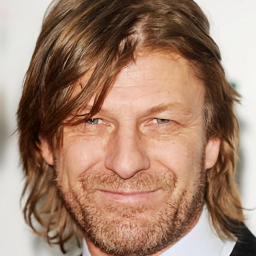}
&
\includegraphics[width=0.125\linewidth]{figures/face/steps/face_029506/img_step_00000.png}
&
\includegraphics[width=0.125\linewidth]{figures/face/steps/face_029506/img_step_00025.png}
&
\includegraphics[width=0.125\linewidth]{figures/face/steps/face_029506/img_step_00050.png}
&
\includegraphics[width=0.125\linewidth]{figures/face/steps/face_029506/img_step_00075.png}
&
\includegraphics[width=0.125\linewidth]{figures/face/steps/face_029506/img_step_00100.png}
&
\includegraphics[width=0.125\linewidth]{figures/face/steps/face_029506/img_step_00150.png}
&
\includegraphics[width=0.125\linewidth]{figures/face/steps/face_029506/img_step_00200.png}
&
\includegraphics[width=0.125\linewidth]{figures/face/steps/face_029506/img_step_00400.png}
\\

\includegraphics[width=0.125\linewidth]{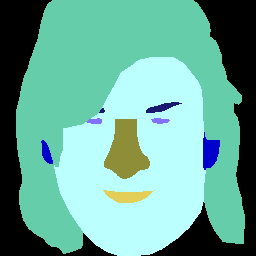}
&
\includegraphics[width=0.125\linewidth]{figures/face/steps/face_029506/label_step_00000.png}
&
\includegraphics[width=0.125\linewidth]{figures/face/steps/face_029506/label_step_00025.png}
&
\includegraphics[width=0.125\linewidth]{figures/face/steps/face_029506/label_step_00050.png}
&
\includegraphics[width=0.125\linewidth]{figures/face/steps/face_029506/label_step_00075.png}
&
\includegraphics[width=0.125\linewidth]{figures/face/steps/face_029506/label_step_00100.png}
&
\includegraphics[width=0.125\linewidth]{figures/face/steps/face_029506/label_step_00150.png}
&
\includegraphics[width=0.125\linewidth]{figures/face/steps/face_029506/label_step_00200.png}
&
\includegraphics[width=0.125\linewidth]{figures/face/steps/face_029506/label_step_00400.png}

\\
\includegraphics[width=0.125\linewidth]{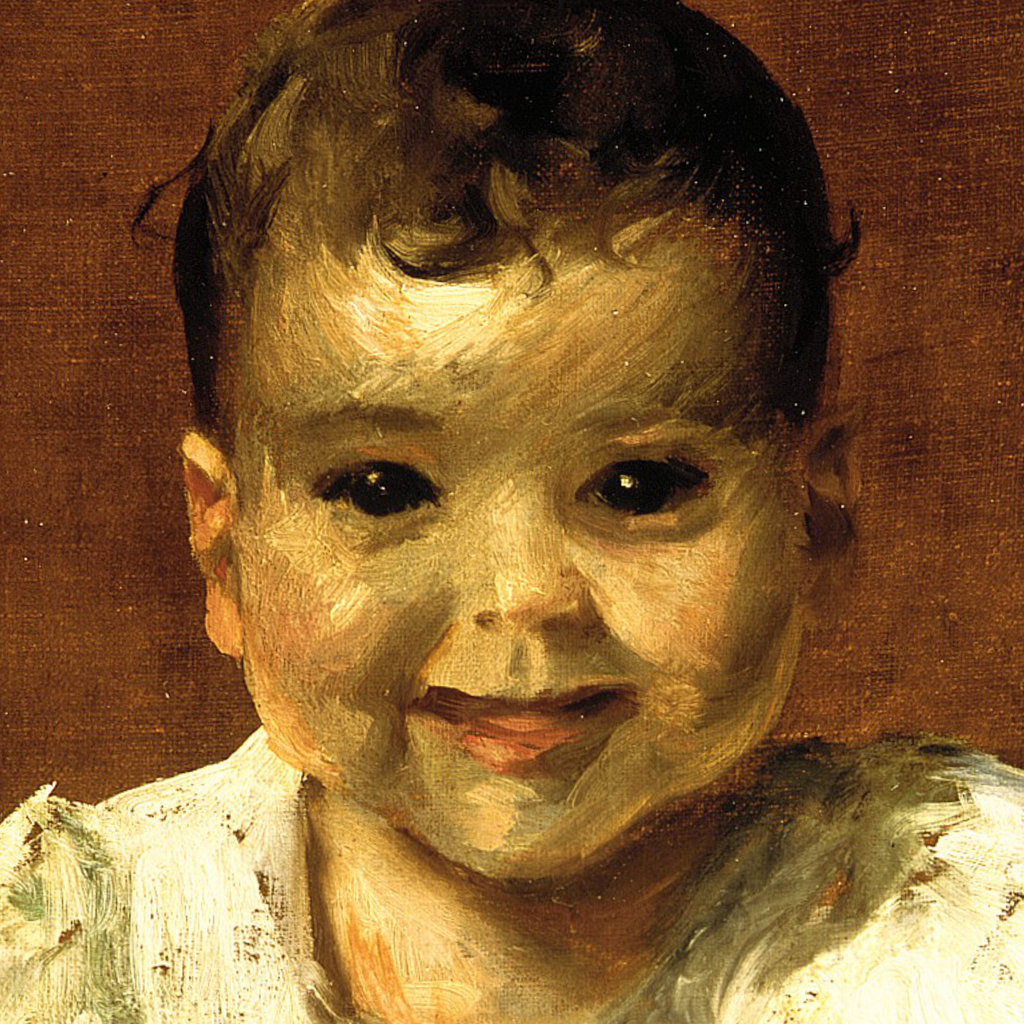}
&
\includegraphics[width=0.125\linewidth]{figures/face/steps/10474-00/img_step_00000.png}
&
\includegraphics[width=0.125\linewidth]{figures/face/steps/10474-00/img_step_00025.png}
&
\includegraphics[width=0.125\linewidth]{figures/face/steps/10474-00/img_step_00050.png}
&
\includegraphics[width=0.125\linewidth]{figures/face/steps/10474-00/img_step_00075.png}
&
\includegraphics[width=0.125\linewidth]{figures/face/steps/10474-00/img_step_00100.png}
&
\includegraphics[width=0.125\linewidth]{figures/face/steps/10474-00/img_step_00150.png}
&
\includegraphics[width=0.125\linewidth]{figures/face/steps/10474-00/img_step_00200.png}
&
\includegraphics[width=0.125\linewidth]{figures/face/steps/10474-00/img_step_00400.png}
\\

\includegraphics[width=0.125\linewidth]{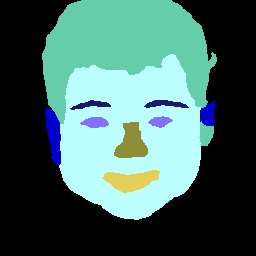}
&
\includegraphics[width=0.125\linewidth]{figures/face/steps/10474-00/label_step_00000.png}
&
\includegraphics[width=0.125\linewidth]{figures/face/steps/10474-00/label_step_00025.png}
&
\includegraphics[width=0.125\linewidth]{figures/face/steps/10474-00/label_step_00050.png}
&
\includegraphics[width=0.125\linewidth]{figures/face/steps/10474-00/label_step_00075.png}
&
\includegraphics[width=0.125\linewidth]{figures/face/steps/10474-00/label_step_00100.png}
&
\includegraphics[width=0.125\linewidth]{figures/face/steps/10474-00/label_step_00150.png}
&
\includegraphics[width=0.125\linewidth]{figures/face/steps/10474-00/label_step_00200.png}
&
\includegraphics[width=0.125\linewidth]{figures/face/steps/10474-00/label_step_00400.png}
\\

\includegraphics[width=0.125\linewidth]{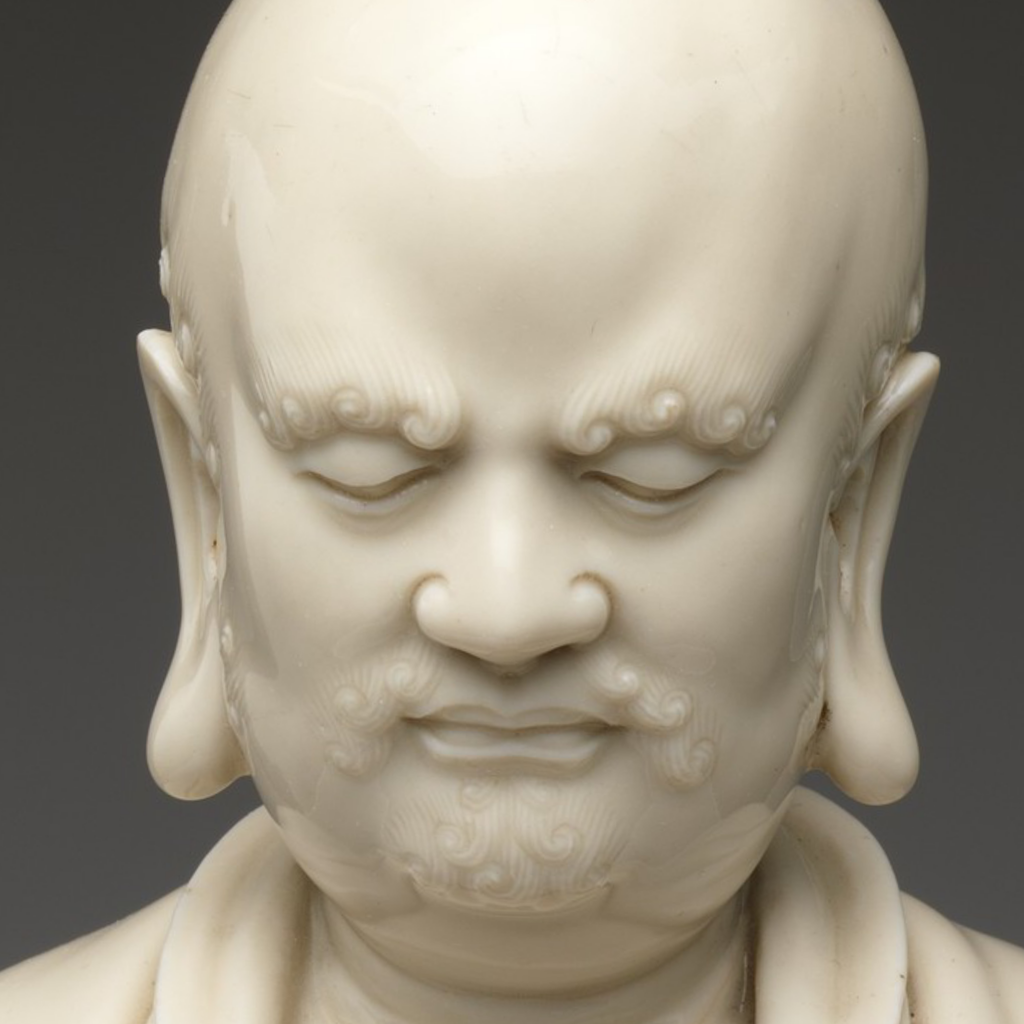}
&
\includegraphics[width=0.125\linewidth]{figures/face/steps/42547-00/img_step_00000.png}
&
\includegraphics[width=0.125\linewidth]{figures/face/steps/42547-00/img_step_00025.png}
&
\includegraphics[width=0.125\linewidth]{figures/face/steps/42547-00/img_step_00050.png}
&
\includegraphics[width=0.125\linewidth]{figures/face/steps/42547-00/img_step_00075.png}
&
\includegraphics[width=0.125\linewidth]{figures/face/steps/42547-00/img_step_00100.png}
&
\includegraphics[width=0.125\linewidth]{figures/face/steps/42547-00/img_step_00150.png}
&
\includegraphics[width=0.125\linewidth]{figures/face/steps/42547-00/img_step_00200.png}
&
\includegraphics[width=0.125\linewidth]{figures/face/steps/42547-00/img_step_00400.png}
\\

\includegraphics[width=0.125\linewidth]{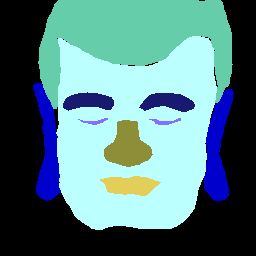}
&
\includegraphics[width=0.125\linewidth]{figures/face/steps/42547-00/label_step_00000.png}
&
\includegraphics[width=0.125\linewidth]{figures/face/steps/42547-00/label_step_00025.png}
&
\includegraphics[width=0.125\linewidth]{figures/face/steps/42547-00/label_step_00050.png}
&
\includegraphics[width=0.125\linewidth]{figures/face/steps/42547-00/label_step_00075.png}
&
\includegraphics[width=0.125\linewidth]{figures/face/steps/42547-00/label_step_00100.png}
&
\includegraphics[width=0.125\linewidth]{figures/face/steps/42547-00/label_step_00150.png}
&
\includegraphics[width=0.125\linewidth]{figures/face/steps/42547-00/label_step_00200.png}
&
\includegraphics[width=0.125\linewidth]{figures/face/steps/42547-00/label_step_00400.png}
\\

\end{tabular}
\end{adjustbox}
\vspace{-4mm}
\caption{\footnotesize \textbf{Face Parts Segmentation Optimization Results.} Image reconstructions and segmentation label predictions at different steps during the optimization process. Step 0 corresponds to using the latent code predicted by the encoder without any further optimization. The model was trained on CelebA-Mask data. Hence, the first example corresponds to in-domain data, while the other two examples, from the MetFace dataset, are out-of-domain cases.}
\label{fig:face-opt}
\end{figure*}
