# Supplementary material for: Semantic Segmentation with Generative Models: Semi-Supervised Learning and Strong Out-of-Domain Generalization
Source: arXiv:2104.05833 source file (2021-04-12)
Supplement: Supplementary file 9 [file face-ablation.tex]

\begin{figure*}[th!]
\begin{adjustbox}{width=0.9\linewidth, center}

\begin{tabular}{cc}

\includegraphics[width=0.45\linewidth]{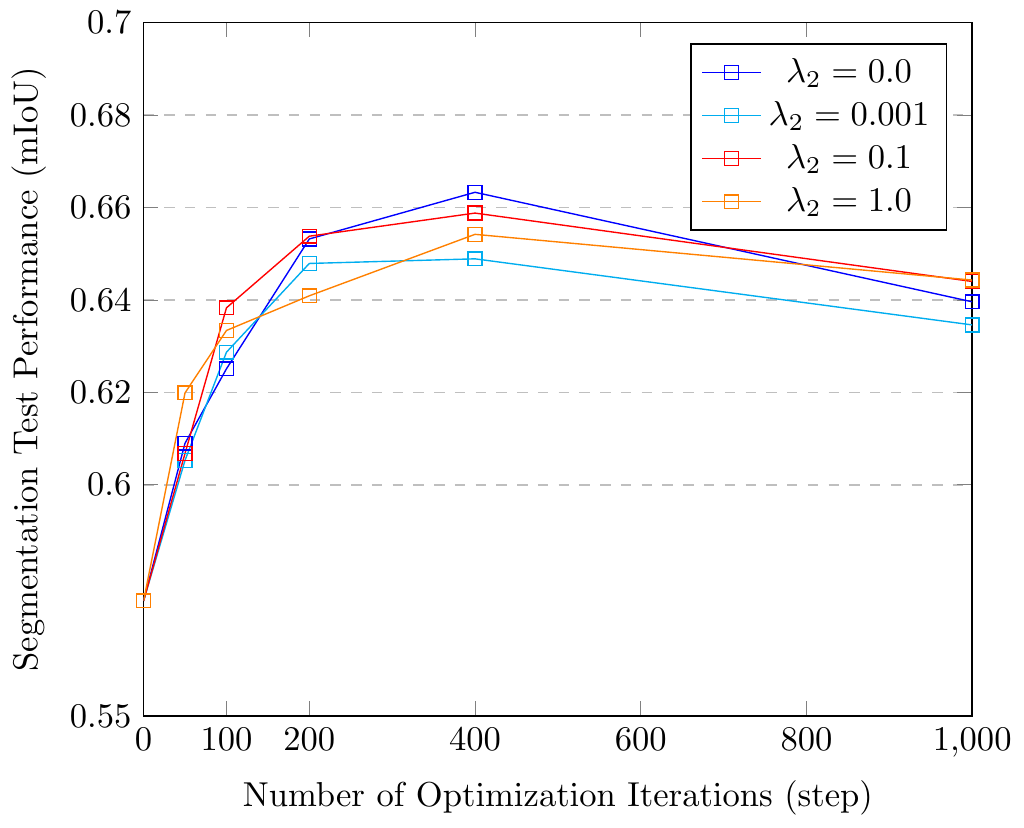}
&
\includegraphics[width=0.45\linewidth]{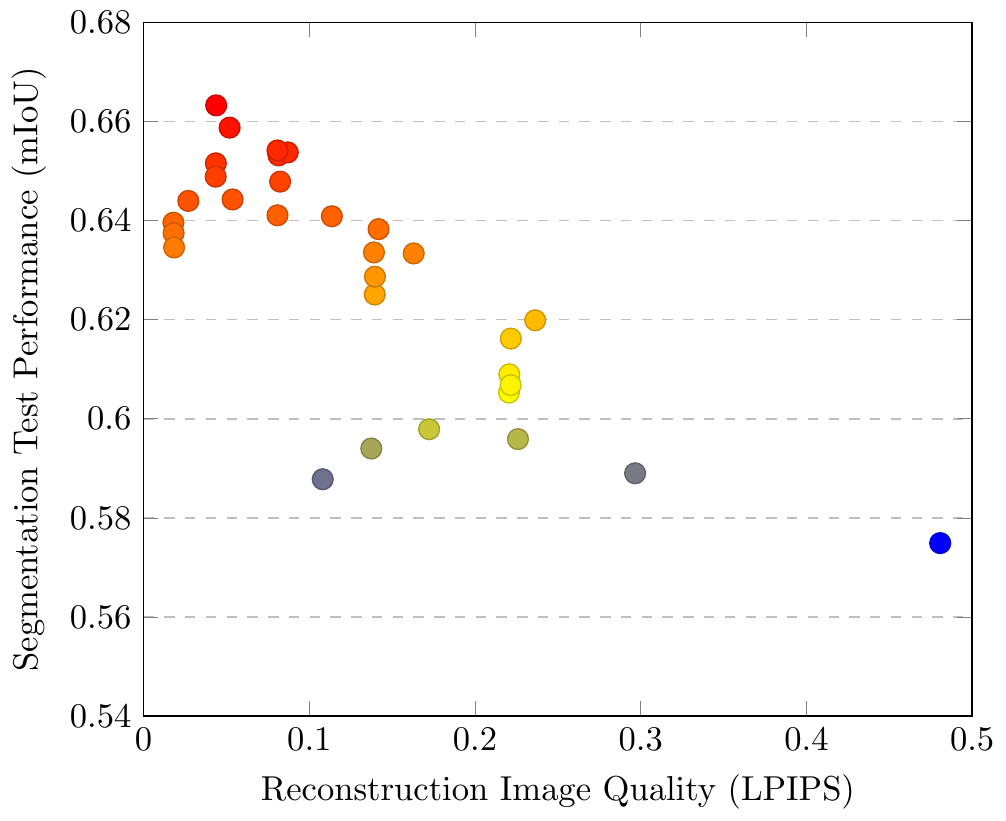}

\end{tabular}
\end{adjustbox}
%\vspace{-4mm}
\caption{\footnotesize \textbf{Optimization Parameter Ablation Study.} \textit{Left:} Ablation study on the number of optimization steps performed during test-time optimization for embedding inference, as well as on the $\lambda_2$ hyperparameter. \textit{Right:} Image reconstruction quality measured in LPIPS against segmentation performance. Segmentation performance is calculated as mIoU on the out-of-domain MetFace dataset. The model for these experiments is trained with 1500 CelebA-Mask labels.}
\label{fig:ablation-opt}
%\vspace{-6mm}
\end{figure*}
